# Supplementary material for: Automata-based Quantitative Verification
Source: arXiv:2010.02055 source file (2020-10-05)
Supplement: Supplementary file 2 [file Appendix.tex]

\renewcommand{\max}{\mu}

\section{Limsup comparator construction}

Formal construction of the limsup comparator is given here. 
Suppose all sequences are natural number sequences, bounded by $\mu$.
The limsup comparator is the B\"uchi automaton $ \LSAut = (\Statess, \Sigma, \delta, \StartState, \Final) $ where
\begin{itemize}
	
	\item $ \Statess = \{s\}  \cup \{s_0, s_1 \dots, s_{ \max}\} \cup \{f_0, f_1 \dots, f_{ \max}\}$
	% where \\ 
	%$ \StartState = \{s\} $, \\
	%$\AcceptingStates = \{(x,c) ||x| \leq \MaxX, 0 \leq c \leq \MaxC \} $, and \\
	%$S_{\bot} = \{(x, \bot) | | x| \leq \MaxX\}$ where $\bot$ is a special character\\
	%where $ x $ and $ c $ are of the form $ \frac{m}{q} $ for integral values of $ m $.
	
	\item $ \Sigma = \{(a,b) : 0 \leq a, b \leq \max \} $ where $ a $ and $ b $ are integers.
	
	\item $\delta \subseteq \Statess\times\Sigma\times \Statess$ is defined as follows:
	\begin{enumerate}
		\item Transitions from start state $ s $:
		$ (s ,(a,b), p) $ for all $(a,b)\in \Sigma$, and for all $p \in \{s\} \cup \{f_0, f_1, \dots, f_{\max}\}$.
		
		\item  Transitions between $f_k$ and $s_k$ for each $k$: 
		\begin{enumerate}[label = \roman*]
			\item $(f_k, \alpha , f_k)$ for $\alpha \in \{k\} \times \{0,1, \dots k\}$.
			\item $(f_k, \alpha , s_k)$ for $\alpha \in \{0,1,\dots k-1\} \times \{0,1, \dots k\}$.
			\item $(s_k, \alpha , s_k)$ for $\alpha \in \{0,1,\dots k-1\} \times \{0,1, \dots k\}$.
			\item $(s_k, \alpha , f_k)$ for $\alpha \in \{k\} \times \{0,1, \dots k\}$.
		\end{enumerate}
		
	\end{enumerate}
	
	\item $ \StartState = \{s\} $
	
	\item $ \Final =  \{f_0, f_1 \dots, f_{ \max}\}$
	% \{(x,c) | 0\leq |x| \leq \MaxX, 0 \leq c \leq \MaxC \} $
	
\end{itemize}

\section{Limit Average Comparator}

\begin{lem}
	\label{lem:sameAverage}
	Let $\Sigma = \{0, 1\dots \mu\}$. Let $L \in \Sigma^*$ s.t. the limit-average of all words in the language $L^{\omega}$ exists. 
	Then average of all words in $L $ is the same. 
	
	%Let $L$ be a regular language over finite words. Then $L^{\omega}$ will consist of words for which limit-average exists then the average of all words in $L$ is the same. 
\end{lem}

\begin{proof}
	Suppose it is possible that two finite words $v_1$, $v_2\in L$ have different average. Let their length be $l_1$ and $l_2$ respectively with the average $a_1$ and $a_2$ respectively where $a_1 \neq a_2$. 
	We will show the presence of a word $w \in L^{\omega}$ s.t. the limit-average of $w$ does not exist.
	
	Let $w_1 = v_1$. Then $\Av{w_1} = a_1$. Next, let $j_2$ be large enough to construct $w_2 = w_i v_2^{j_2}$ such that $\Av{w_2}\approx a_2$. Next, let $j_3$ be large enough to construct $w_3 = w_2 v_1^{j_3}$ such that $\Av{w_3} \approx a_1$. 
	Continue constructing $w_4, w_5 \dots$ in a similar fashoin s.t. their average change between  $a_2, a_1 \dots$ respectively. 
	
	Let these $w = w_n$ as $n\rightarrow \infty$. Then $w \in L^{\omega}$, and since the average of its finite-length prefixes keeps changing between $a_1$ and $a_2$, limit-average of $w$ does not exist. 
	
	This contradicts the premise that the limit-average of all words in $L^{\omega}$ exists. Therefore, our assumption that words $v_1$ and $v_2$ can have different average has been contradicted. 
	
\end{proof}

\begin{lem}
	\label{lem:sameLA}
	Let $\Sigma = \{0, 1, \dots \mu \}$. Let $L\subseteq \Sigma^*$ s.t. the average of all words in $\Sigma$ is the same, say $a$.	
	Let $w \in L^{\omega}$ s.t. limit-average of  $w$ exists. Then $\LA{w} = a$ 
\end{lem}
\begin{proof}
Let $w = w_1w_2w_3\dots$. There exists infinitely many prefixes of $w$, prefix $w[i] = w_1w_2\dots w_i$ s.t. $\Av{w[i]} = a$.
Since we are given  that the limit-average of $w$ exists, it must be equal to $a$.
\end{proof}

\paragraph{\bf Theorem~\ref{Lemma:LARegularNotExist}}
	
	Let $\Sigma = \{0,1\dots, \mu\}$. Let $\L_{LA} \subseteq \Sigma^{\omega}$.
	$\L_{LA}$ is neither an $\omega$-regular nor an $\omega$-context-free language.
