# Supplementary material for: Automata-based Quantitative Verification
Source: arXiv:2010.02055 source file (2020-10-05)
Supplement: Supplementary file 3 [file Appendix.tex]

\section{Appendix}

\subsection{Universal comparator: Missing proofs}

\renewcommand{\MaxC}{\mu_C}
\renewcommand{\MaxX}{\mu_X}

\begin{lemma}
 \label{Lemma:discount-invariant1A}
 {\rm \bf(Lemma~\ref{Lemma:discount-invariant1A} from main paper)}
Let $V, C, X$ be the number sequences, $ d > 1 $ be a positive integer such that following equations holds true:
 \begin{enumerate}
 \item  \label{eq:initial} When $ i = 0 $, $ V[0] + C[0] + X[0] = 0$
 \item \label{eq:invariant} When $ i\geq 1 $, $V[i] + C[i] + X[i] = d \cdot X[i-1]$
 \end{enumerate}
 Then $ \DSum{V}{d} + \DSum{C}{d} =0$.
 \end{lemma}
 \begin{proof}

 This follows proof by expansion of all terms. Specifically, expand out $\DSum{V}{d} + \DSum{C}{d}$ to $\Sigma_{i=0}^{\infty} \frac{(V[i] + C[i])}{d^i}$ and replace each (V[i] + C[i]) with substitutions given by the equations. All terms will cancel each other to get $\DSum{V}{d} + \DSum{C}{d}  = 0$. 
 \end{proof}
 The following result has been taken  from ~\cite{BCVFoSSaCS18} as it is:
 \begin{lemma}{\rm ~\cite{BCVFoSSaCS18}}
	\label{lemma:FiniteAlphabetXandC}
	Let $d>1$ be an integer discount-factor. Let $A$ and $B$ be nonnegative
	integer sequences bounded by $\mu$ s.t. $\DSum{A}{d} <
	\DSum{B}{d}$. Let C and X be sequences s.t.
    
    \begin{enumerate}
 \item  \label{eq:initial} When $ i = 0 $, $ A[0] + C[0] + X[0] = B[0]$
 \item \label{eq:invariant} When $ i\geq 1 $, $A[i] + C[i] + X[i] = B[i] + d \cdot X[i-1]$
 \end{enumerate}
 There exists at least one pair of integer-sequences $C$ and $X$ that satisfy the following two equations
	\begin{enumerate}
		\item For all $i \geq 0$, $0 \leq C[i] \leq \mu\cdot \frac{d}{d-1}$. and
		\item For all $i \geq 0$, $0 \leq |X[i]| \leq 1 + \frac{\mu}{d-1}$
	\end{enumerate} 
\end{lemma}
Lemma~\ref{lemma:FiniteAlphabetXandC} can we reworded in our context by replacing each $(A[i] - B[i])$ with $V[i]$ and using Lemma~\ref{Lemma:discount-invariant1A} as follows:
 \begin{lemma}
	\label{lemma:mybounds}
	Let $d>1$ be an integer discount-factor. Let $V$
	integer sequences bounded by $\mu$ s.t. $\DSum{V}{d} < 0 $. Let C and X be as constructed in Lemma~\ref{Lemma:discount-invariant1A}. There exists at least one pair of integer-sequences $C$ and $X$ that satisfy the following two equations
	\begin{enumerate}
		\item For all $i \geq 0$, $0 \leq C[i] \leq \mu\cdot \frac{d}{d-1}$. and
		\item For all $i \geq 0$, $0 \leq |X[i]| \leq 1 + \frac{\mu}{d-1}$
	\end{enumerate} 
\end{lemma}
Let $\MaxC = \mu\cdot \frac{d}{d-1}$, and $\MaxX  = 1 + \frac{\mu}{d-1}$
 \begin{lemma}
	\label{lemma:RemoveCA}{\rm \bf(Lemma~\ref{lemma:RemoveC} from main paper)}
	Let $V$ and be an integer-sequence bounded by $\mu$ s.t. $\DSum{V}{d} \leq 0$, and $X$ be an integer sequence bounded by $(1 + \frac{\mu}{d-1})$, then there exists an $X$ s.t. the following is true:
	\begin{enumerate}
		\item \label{eq:initialRemoveC} When $i=0$, $0\leq -(X[0] + V[0]) \leq \mu\cdot\frac{d}{d-1}$
		\item  \label{eq:invariantRemoveC} When $i\geq 1$, $ 0\leq (d \cdot X[i-1] - V[i] - X[i] )\leq  \mu\cdot\frac{d}{d-1}$
	\end{enumerate}
	
\end{lemma}
\begin{proof}
The proof for this lemma combines Lemma~\ref{Lemma:discount-invariant1A} and Lemma~\ref{lemma:mybounds}. 

Let $V$, $C$ and $X$ be bounded sequences that satisfy the equations from Lemma~\ref{Lemma:discount-invariant1A}. Then, the equations can be re-written as
\begin{enumerate}
 \item  \label{eq:initial} When $ i = 0 $, $ C[0] = -V[0] + X[0] $
 \item \label{eq:invariant} When $ i\geq 1 $, $C[i] = d \cdot X[i-1] - V[i] - X[i]$
 \end{enumerate}
 Furthermore, since $\DS{V}{d} < 0$, we know that there exists integer sequences $X$ and $C$ that s.t $0\leq C[i] \leq \MaxC$ and $|X[i]| \leq \MaxX$ (Lemma~\ref{lemma:mybounds}). Then, for that sequence $X$,  by we get the desired bounds by applying the bound on $C[i]$ to the equations above. 
\end{proof}
